# Supplementary material for: Surface Reconstructions in Thin-Films of Magnetic Topological Insulator MnBi$_2$Te$_4$
Source: arXiv:2501.11176 source file (2025-01-19)
Supplement: Supplementary file 1 [file MnBiTe_SI.pdf]

# Supporting Information

# Surface Reconstructions in Thin-Films of Magnetic Topological Insulator $MnBi_2Te_4$

Shahid Sattar,*,† Daniel Hedman,‡ and C. M. Canali†

†*Department of Physics and Electrical Engineering, Linnaeus University, SE-39231 Kalmar, Sweden*

‡*Center for Multidimensional Carbon Materials (CMCM), Institute for Basic Science (IBS), Ulsan 44919, Republic of Korea*

E-mail: shahid.sattar@lnu.se

# Computational Details

To correctly describe strong on-site Coulomb interactions of localized Mn $d-$electrons, we used Hubbard $U$ correction (GGA+U method) following Dudarev's scheme[1] and fixed the onsite Coulomb (U) and exchange (J) parameters to the value of 3.9 eV and 0.0 eV, respectively. We always used a vacuum layer of 15 Å, in the out-of-the-plane direction to prevent periodic-image interactions. A real-space tight binding Hamiltonian was obtained based on maximally localized Wannier functions (MLWFs) using the Wannier90 package.[2–4] For this purpose, we used the VASP2WANNIER90 interface and included Mn$-d$, Se$-p$ and Te$-p$ orbitals in generating the Wannier functions. Topological characteristics were computed using the WannierTools package,[5] whereas Chern number ($\mathcal{C}$) was evaluated by tracking the evolution of hybrid Wannier functions as implemented in Z2pack.[6,7]

The machine learning force fields (MLFFs) were constructed on-the-fly using *ab-initio* molecular dynamics (MD) simulations combined with a Bayesian learning algorithm, as implemented in VASP.[8–10] Initially, on-the-fly MLFF-accelerated *ab-initio* MD simulations were performed over temperature ranges of 5 to 600 K and later, from 600 K to 900 K to generate the training dataset. During these simulations, high-error structures are automatically identified and sampled, ensuring a comprehensive training dataset. The training data obtained was then used to refit the VASP MLFF, resulting in a much faster force field capable of driving MD simulations for a longer time of ∼35 ns. The refined MLFF was subsequently employed to perform production MD simulations. Specifically, four independent heating simulations were conducted from 5 to 400 K, and another four were conducted from 400 to 700 K, each using a constant heating rate of 20 K/ns. All MD simulations were carried out in the canonical (NVT) ensemble, utilizing a Nosé-Hoover-chain thermostat[11] with a characteristic time scale of 100 ps to regulate temperature. For studying energy barriers and reaction pathways between different reconstructed and non-reconstructed MBT thin films, nudged elastic band (NEB) calculations were performed[12] with 6-8 images between the initial and final states. Finally, vaspkit[13] and pyprocar[14] packages were employed for pre- or

post-processing and plotting of the data.

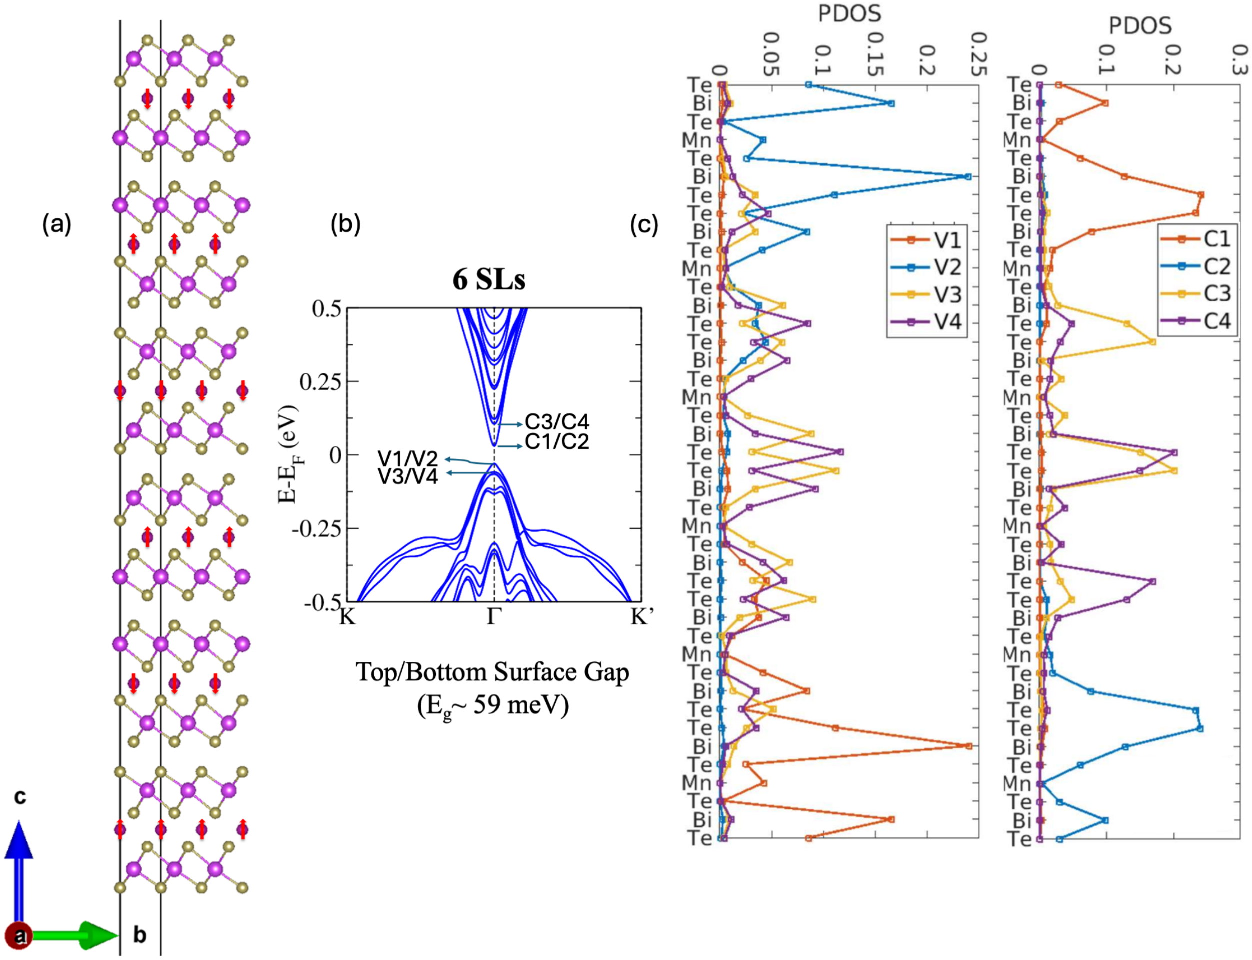


Figure S1: (a) Crystal structure of a 6 SL $MnBi_2Te_4$ thin film having homogeneous in-plane ferromagnetic order by the Mn-atoms and out-of-plane antiferromagnetic ordering between the constituent layers. (b) Electronic band-structure showing a top/bottom surface gap of 59 meV. Doubly degenerate top-most doubly valence bands V1/V2 and V3/V4 and conduction bands C1/C2 and C3/C4 are explicitly labelled. (c) Partial density-of-states (PDOS) projected on all atoms of 6-SL for topmost valence and bottom-most conduction bands. PDOS clearly indicates that the main contribution close to Fermi-energy is coming from V1-V4 and C1-C4 bands.

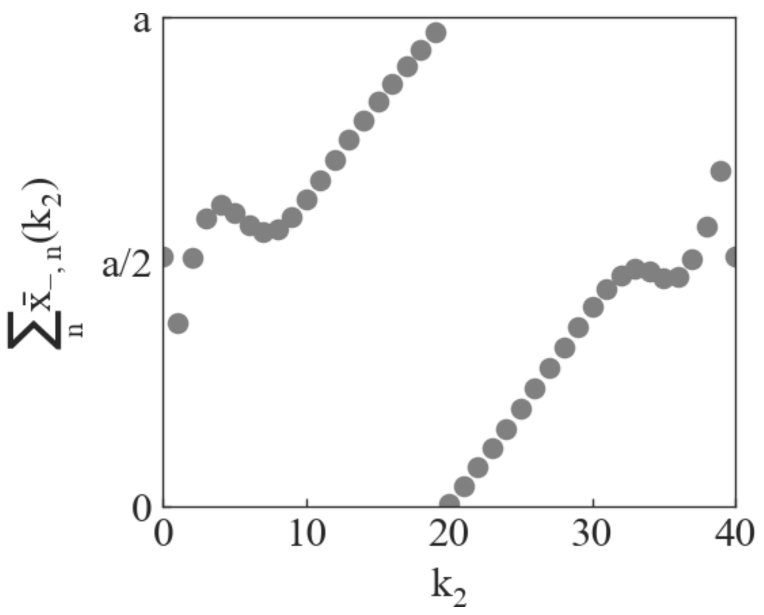


Figure S2: Spin-Resolved Wannier Charge Center for a 6-SL $MnBi_2Te_4$ thin film.

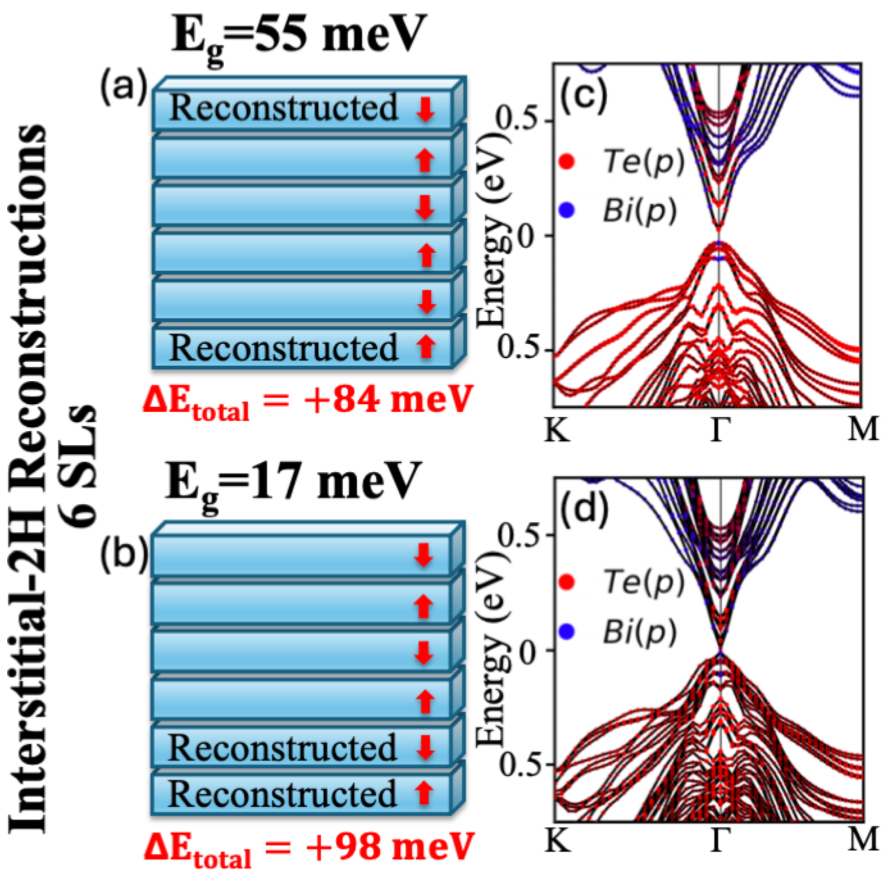


Figure S3: (a) Sketch of Interstitial-2H surface reconstructions for 6-SL MBT thin film and their atom- and orbital-projected electronic band structures showing band inversions.

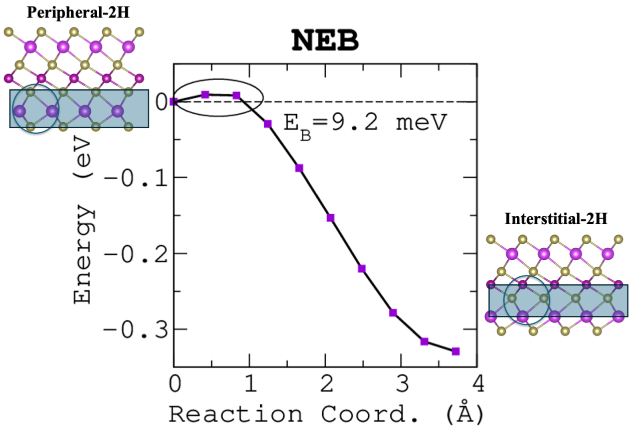


Figure S4: Nudged elastic band (NEB) calculations showing a small energy barrier between peripheral-2H and interstitial-2H surface reconstructions.

# Energy Barriers between Non-reconstructed and Reconstructed MBT thin films

We performing nudged elastic band (NEB) calculations to study energy barrier and reaction pathway between MBT non- and reconstructed thin films. First, despite a total energy difference of 335 meV between initial state (peripheral-2H) to final state (interstitial-2H) reconstructions, our nudged elastic band (NEB) calculations show that an energy barrier of 9.2 meV exists in going from peripheral-2H to interstitial-2H surface reconstruction, as shown in the Figure S4.

For the second case, our calculations reveal that albeit an interstitial-2H reconstructed MBT surface is only 40 meV higher in energy than the non-reconstructed $MnBi_2Te_4$, yet there exists a large energy barrier of $\approx$1.9 eV which prohibits transformation of the former to the latter, as shown in the Figure S5.

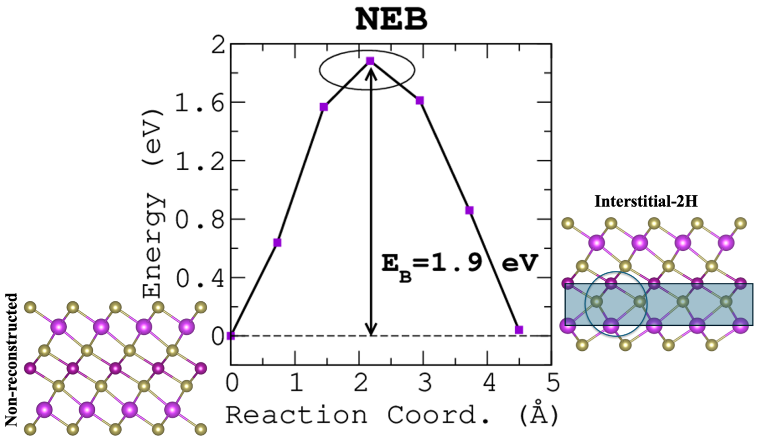


Figure S5: Nudged elastic band (NEB) calculation showing a large energy barrier of 1.9 eV between interstitial-2H and non-reconstructed MBT surface.

# Spin Hall Conductivity for Peripheral-2H Reconstruction

We have calculated spin Hall conductivity (SHC) for peripheral-2H reconstructed 6-SL MBT thin film using Kubo's formalism as given by the following expressions,[15–17]

$$\sigma^z_{xy} = \frac{e^2}{\hbar} \sum_{n \neq n'} \frac{dk}{(2\pi)^2} [f(E_{n,k}) - f(E_{n',k})] \Omega^z_{n,xy}(k), \tag{1}$$

and

$$\Omega^z_{n,xy}(k) = -2\hbar^2 Im \sum_{\substack{n=occ,\\ n'=unocc}} \frac{\langle u_{nk}|j^z_x|u_{n'k}\rangle \langle u_{n'k}|\hat{v}_y|u_{nk}\rangle}{(E_{n,k} - E_{n',k})^2}$$

Here, $E_{n,k}$ is the eigenvalue of the bloch function $|u_{nk}\rangle$, $f(E_{n,k})$ is the Fermi-Dirac distribution function. Besides, $j^z_x$ and $\hat{v}_y$ are spin current and velocity operators, respectively. A non-zero SHC conductivity for peripheral-2H reconstructed 6-SL MBT confirms the topological nature of this system, as shown in the Figure S6.

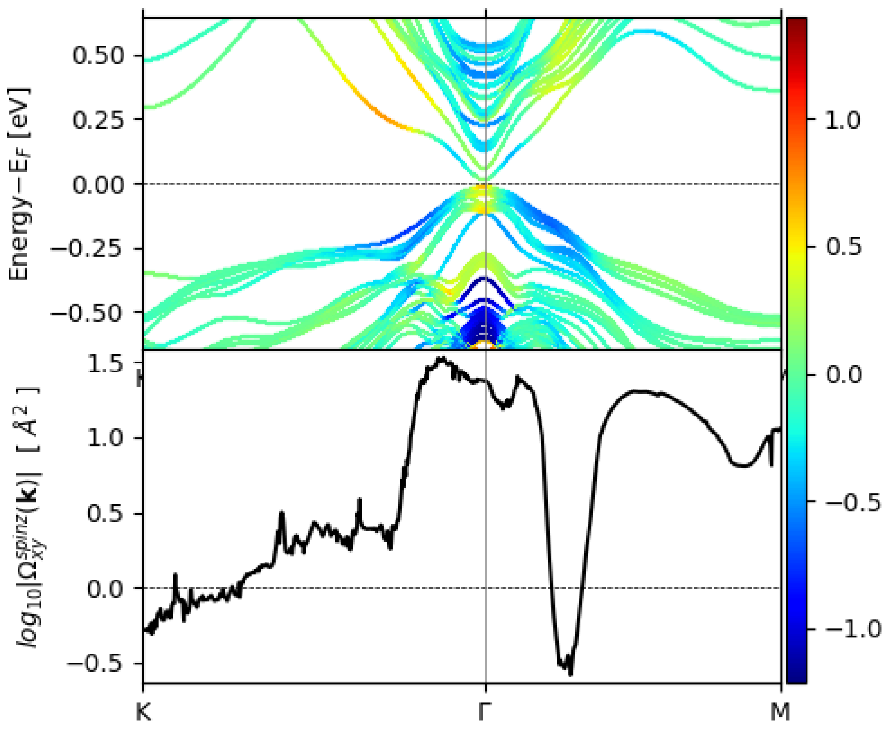


Figure S6: Spin-Hall conductivity for peripheral-2H reconstructed 6-SL MBT surface.

# References


(1) Dudarev, S. L.; Botton, G. A.; Savrasov, S. Y.; Humphreys, C.; Sutton, A. P. Electron-energy-loss spectra and the structural stability of nickel oxide: An LSDA+ U study. *Physical Review B* **1998**, *57*, 1505.

(2) Marzari, N.; Vanderbilt, D. Maximally localized generalized Wannier functions for composite energy bands. *Physical Review B* **1997**, *56*, 12847.

(3) Mostofi, A. A.; Yates, J. R.; Pizzi, G.; Lee, Y.-S.; Souza, I.; Vanderbilt, D.; Marzari, N. An updated version of wannier90: A tool for obtaining maximally-localised Wannier functions. *Computer Physics Communications* **2014**, *185*, 2309–2310.

(4) Pizzi, G.; Vitale, V.; Arita, R.; Blügel, S.; Freimuth, F.; Géranton, G.; Gibertini, M.; Gresch, D.; Johnson, C.; Koretsune, T.; others Wannier90 as a community code: new features and applications. *Journal of Physics: Condensed Matter* **2020**, *32*, 165902.

(5) Wu, Q.; Zhang, S.; Song, H.-F.; Troyer, M.; Soluyanov, A. A. WannierTools: An open-source software package for novel topological materials. *Computer Physics Communications* **2018**, *224*, 405–416.

(6) Gresch, D.; Autes, G.; Yazyev, O. V.; Troyer, M.; Vanderbilt, D.; Bernevig, B. A.; Soluyanov, A. A. Z2Pack: Numerical implementation of hybrid Wannier centers for identifying topological materials. *Physical Review B* **2017**, *95*, 075146.

(7) Soluyanov, A. A.; Vanderbilt, D. Computing topological invariants without inversion symmetry. *Physical Review B* **2011**, *83*, 235401.

(8) Jinnouchi, R.; Lahnsteiner, J.; Karsai, F.; Kresse, G.; Bokdam, M. Phase Transitions of Hybrid Perovskites Simulated by Machine-Learning Force Fields Trained on the Fly with Bayesian Inference. *Physical review letters* **2019**, *122*, 225701.

(9) Jinnouchi, R.; Karsai, F.; Kresse, G. On-the-fly machine learning force field generation: Application to melting points. *Physical Review B* **2019**, *100*, 014105.

(10) Jinnouchi, R.; Karsai, F.; Verdi, C.; Asahi, R.; Kresse, G. Descriptors representing two- and three-body atomic distributions and their effects on the accuracy of machine-learned inter-atomic potentials. *The Journal of chemical physics* **2020**, *152*, 234102.

(11) Martyna, G. J.; Klein, M. L.; Tuckerman, M. Nosé–Hoover chains: The canonical ensemble via continuous dynamics. *The Journal of Chemical Physics* **1992**, *97*, 2635–2643.

(12) Mills, G.; Jónsson, H.; Schenter, G. K. Reversible work transition state theory: application to dissociative adsorption of hydrogen. *Surface Science* **1995**, *324*, 305–337.

(13) Wang, V.; Xu, N.; Liu, J.-C.; Tang, G.; Geng, W.-T. VASPKIT: A user-friendly interface facilitating high-throughput computing and analysis using VASP code. *Computer Physics Communications* **2021**, *267*, 108033.

(14) Herath, U.; Tavadze, P.; He, X.; Bousquet, E.; Singh, S.; Muñoz, F.; Romero, A. H. PyProcar: A Python Library for Electronic Structure Pre/Post-Processing. *Comput. Phys. Commun.* **2020**, *251*, 107080.

(15) Matthes, L.; Küfner, S.; Furthmüller, J.; Bechstedt, F. Intrinsic spin Hall conductivity in one-, two-, and three-dimensional trivial and topological systems. *Physical Review B* **2016**, *94*, 085410.

(16) Sun, Y.; Zhang, Y.; Felser, C.; Yan, B. Strong intrinsic spin Hall effect in the TaAs family of Weyl semimetals. *Physical Review Letters* **2016**, *117*, 146403.

(17) Qiao, J.; Zhou, J.; Yuan, Z.; Zhao, W. Calculation of intrinsic spin Hall conductivity by Wannier interpolation. *Physical Review B* **2018**, *98*, 214402.
